# Supplementary material for: Uncovering the Source of Machine Bias
Source: arXiv:2201.03092 source file (2022-01-09)
Supplement: Supplementary file 1 [file appendix.tex]

In the appendix, we describe our bayesian version model. The difference of this model with the one in Section~\ref{sec:model} is the belief updating process when observing new signals.

Because all these signals are highly nonnormal, in order to implement Bayesian updating rules with normal-normal conjugate families, we use Box-Cox transformation to tranform them to nearly normal distributions. All these signals have a mass concentration at zero. We add 1 to these signals since the Box-Cox likelihood does not behave well at zero.
After transformation, assume all these signals follow normal distributions around their corresponding means:

\begin{equation}
\begin{aligned}
    \frac{(1+D_{it})^{\alpha}-1}{\alpha} &= D_i^M + \omega_{it},~\omega_{it} \sim N(0, \sigma_\omega^2), \\
    \frac{(1+M_{it})^{\gamma}-1}{\gamma} &= M_i^M + \nu_{it},~\nu_{it} \sim N(0, \sigma_\nu^2), \\
    \frac{(1+A_{it})^{\delta}-1}{\delta} &= A_i^M + \varpi_{it},~\varpi_{it} \sim N(0, \sigma_\varpi^2), \\
    \frac{(1+H_{it})^{\theta}-1}{\theta} &= H_i^M + \upsilon_{it},~\upsilon_{it} \sim N(0, \sigma_\upsilon^2),
\label{eq:signal-mean}
\end{aligned}
\end{equation}

\noindent where $\alpha, \gamma, \delta, \theta$ are the Box-Cox parameters, and $D_i^M$, $M_i^M$, $A_i^M$ and $H_i^M$ are the means of person $i$'s four signals, and $\omega_{it}, \nu_{it}, \varpi_{it}, \upsilon_{it}$ are stochastic terms that are i.i.d. over time. The evaluators believe that all these signals are related to the credit quality in the following way:

\begin{equation}
\begin{aligned}
    D_i^M &= D_0 + \phi Q_i + \eta_i, \\
    M_i^M &= M_0 + \varphi Q_i + \zeta_i, \\
    A_i^M &= A_0 + \psi Q_i + \varsigma_i, \\
    H_i^M &= H_0 + \rho Q_i + \iota_i,
\label{eq:signal-mean-quality}
\end{aligned}
\end{equation}

\noindent where $\phi$, $\varphi$, $\psi$ and $\rho$ are parameters, and $\eta_i$, $\zeta_i$, $\varsigma_i$ and $\iota_i$ are deviations which follow i.i.d normal distributions, i.e. $\eta_i \sim N(0, \sigma_\eta^2)$, $\zeta_i \sim N(0, \sigma_\zeta^2)$, $\varsigma_i \sim N(0, \sigma_\varsigma^2)$ and $\iota_i \sim N(0, \sigma_\iota^2)$. 
%{\color{red} For identification, $\eta_I = \sum_{i=1}^{I-1}\eta_i, \zeta_I = \sum_{i=1}^{I-1}\zeta_i, \varsigma_I = \sum_{i=1}^{I-1}\varsigma_i, \iota_I = \sum_{i=1}^{I-1}\iota_i$.}
Combining (\ref{eq:signal-mean}) and (\ref{eq:signal-mean-quality}) we get:

\begin{equation}
\begin{aligned}
    \frac{(1+D_{it})^{\alpha}-1}{\alpha} &= D_0 + \phi Q_i + \eta_i  + \omega_{it}, \\
    \frac{(1+M_{it})^{\gamma}-1}{\gamma} &= M_0 + \varphi Q_i + \zeta_i + \nu_{it}, \\
    \frac{(1+A_{it})^{\delta}-1}{\delta} &= A_0 + \psi Q_i + \varsigma_i + \varpi_{it}, \\
    \frac{(1+H_{it})^{\theta}-1}{\theta} &= H_0 + \rho Q_i + \iota_i + \upsilon_{it},
\label{eq:signal-quality}
\end{aligned}
\end{equation}

At time $t=0$, before observing any repayment behaviors, the evaluator holds prior beliefs for these four signals that each borrower $i$'s repayment behaviors follows normal distributions:

\begin{equation}
\begin{aligned}
    D_i^M &\sim N(D_0 + \phi Q_i^{M}, \phi^2\sigma_{Q_0}^2+\sigma_\eta^2), \\
    M_i^M &\sim N(M_0 + \varphi Q_i^{M}, \varphi^2\sigma_{Q_0}^2+\sigma_\zeta^2), \\
    A_i^M &\sim N(A_0 + \psi Q_i^{M}, \psi^2\sigma_{Q_0}^2+\sigma_\varsigma^2), \\
    H_i^M &\sim N(H_0 + \rho Q_i^{M}, \rho^2\sigma_{Q_0}^2+\sigma_\iota^2).
\end{aligned}
\end{equation}

Denote the $D_{it}^M$, $M_{it}^M$, $A_{it}^M$, $H_{it}^M$ and $Q_{it}$ as the prior means at time $t$.
At time $t=0$, $D_{i0}^M=D_0 + \phi Q_i^{M}$, $M_{i0}^M=M_0 + \varphi Q_i^{M}$, $A_{i0}^M=A_0 + \psi Q_i^{M}$, $H_{i0}^M=H_0 + \rho Q_i^{M}$ and $Q_{i0}=\bm{\beta} \mathbf{X}_i$. Similarly, denote the $\sigma_{D_{it}}^2, \sigma_{M_{it}}^2, \sigma_{A_{it}}^2, \sigma_{H_{it}}^2, $ and $Q_{it}$ as the prior variances at time $t$, and 
$\sigma_{D_{i0}}^2 = \phi^2\sigma_{Q_0}^2+\sigma_\eta^2, 
\sigma_{M_{i0}}^2 = \varphi^2\sigma_{Q_0}^2+\sigma_\zeta^2,
\sigma_{A_{i0}}^2 = \psi^2\sigma_{Q_0}^2+\sigma_\varsigma^2,
\sigma_{H_{i0}}^2 = \rho^2\sigma_{Q_0}^2+\sigma_\iota^2$.

Assume that given $Q_i$, all signals $D_{it}$, $M_{it}$, $A_{it}$ and $H_{it}$ are independent from each other. 
%{\color{orange} PROBLEM: $A$ and $H$ should be dependent on $D$ and $M$, because we can only observe $A$ and $H$ when there are late payments.}
When $i$'s repayment behavior is observed at time $t$, the evaluator updates her perceptions of $D_{it}, M_{it}, A_{it}, H_{it}$ and the credit quality of $Q_{it}$ based on Bayesian rules:

\begin{equation}
\begin{aligned}
    D_{it}^M &= D_{i,t-1}^M + \frac{\sigma_{D_{i,t-1}}^2}{\sigma_{D_{i,t-1}}^2+\sigma_\omega^2}
    (\frac{(1+D_{it})^{\alpha}-1}{\alpha}-D_{i,t-1}^M) \\
    M_{it}^M &= M_{i,t-1}^M + \frac{\sigma_{M_{i,t-1}}^2}{\sigma_{M_{i,t-1}}^2+\sigma_\nu^2}
    (\frac{(1+M_{it})^{\gamma}-1}{\gamma}-M_{i,t-1}^M) \\
    A_{it}^M &= A_{i,t-1}^M + \frac{\sigma_{A_{i,t-1}}^2}{\sigma_{A_{i,t-1}}^2+\sigma_\varpi^2}
    (\frac{(1+A_{it})^{\delta}-1}{\delta}-A_{i,t-1}^M) \\
    H_{it}^M &= H_{i,t-1}^M + \frac{\sigma_{H_{i,t-1}}^2}{\sigma_{H_{i,t-1}}^2+\sigma_\upsilon^2}
    (\frac{(1+H_{it})^{\theta}-1}{\theta}-H_{i,t-1}^M) \\
\end{aligned}
\end{equation}

\begin{equation}
\begin{aligned}
    % Q_{i1} &= Q_{i0} +
    % \frac{\sigma_{Q_0}^2(\sigma_\zeta^2+\sigma_\nu^2)\phi}{(\sigma_\zeta^2+\sigma_\nu^2)(\sigma_\eta^2+\sigma_\omega^2)+\sigma_{Q_0}^2(\sigma_\zeta^2+\sigma_\nu^2)\phi^2+\sigma_{Q_0}^2(\sigma_\eta^2+\sigma_\omega^2)\varphi^2}(D_{i1}-D_{i0}^M) \\
    % &+ \frac{\sigma_{Q_0}^2(\sigma_\eta^2+\sigma_\omega^2)\varphi}{(\sigma_\zeta^2+\sigma_\nu^2)(\sigma_\eta^2+\sigma_\omega^2)+\sigma_{Q_0}^2(\sigma_\zeta^2+\sigma_\nu^2)\phi^2+\sigma_{Q_0}^2(\sigma_\eta^2+\sigma_\omega^2)\varphi^2}(M_{i1}-M_{i0}^M) \\
    Q_{it} = Q_{i,t-1} 
    &  +
    \frac{\frac{\phi^2}{\sigma_\eta^2+\sigma_\omega^2}}{\frac{\phi^2}{\sigma_\eta^2+\sigma_\omega^2} + \frac{\varphi^2}{\sigma_\zeta^2+\sigma_\nu^2} + \frac{\psi^2}{\sigma_\varsigma^2+\sigma_\varpi^2} + \frac{\rho^2}{\sigma_\iota^2+\sigma_\upsilon^2} + \frac{1}{\sigma_{Q_{i,t-1}}^2}}\frac{1}{\phi}
    (\frac{(1+D_{it})^{\alpha}-1}{\alpha}-D_{i,t-1}^M) \\
    &  + \frac{\frac{\varphi^2}{\sigma_\zeta^2+\sigma_\nu^2}}{\frac{\phi^2}{\sigma_\eta^2+\sigma_\omega^2} + \frac{\varphi^2}{\sigma_\zeta^2+\sigma_\nu^2} + \frac{\psi^2}{\sigma_\varsigma^2+\sigma_\varpi^2} + \frac{\rho^2}{\sigma_\iota^2+\sigma_\upsilon^2} + \frac{1}{\sigma_{Q_{i,t-1}}^2}} \frac{1}{\varphi}
    (\frac{(1+M_{it})^{\gamma}-1}{\gamma}-M_{i,t-1}^M) \\
    &  + \frac{\frac{\psi^2}{\sigma_\varsigma^2+\sigma_\varpi^2}}{\frac{\phi^2}{\sigma_\eta^2+\sigma_\omega^2} + \frac{\varphi^2}{\sigma_\zeta^2+\sigma_\nu^2} + \frac{\psi^2}{\sigma_\varsigma^2+\sigma_\varpi^2} + \frac{\rho^2}{\sigma_\iota^2+\sigma_\upsilon^2} + \frac{1}{\sigma_{Q_{i,t-1}}^2}} \frac{1}{\psi}
    (\frac{(1+A_{it})^{\delta}-1}{\delta}-A_{i,t-1}^M) \\
    &  + \frac{\frac{\rho^2}{\sigma_\iota^2+\sigma_\upsilon^2}}{\frac{\phi^2}{\sigma_\eta^2+\sigma_\omega^2} + \frac{\varphi^2}{\sigma_\zeta^2+\sigma_\nu^2} + \frac{\psi^2}{\sigma_\varsigma^2+\sigma_\varpi^2} + \frac{\rho^2}{\sigma_\iota^2+\sigma_\upsilon^2} + \frac{1}{\sigma_{Q_{i,t-1}}^2}} \frac{1}{\rho}
    (\frac{(1+H_{it})^{\theta}-1}{\theta}-H_{i,t-1}^M) \\
\end{aligned}
\end{equation}

Given the four signals observed at time $t$, the evaluator updates these prior variances using Bayesian updating rules for normal-normal conjugate families:

\begin{equation}
\begin{aligned}
     \sigma_{D_{it}}^2 = \frac{1}{\frac{1}{\sigma_{D_{i,t-1}}^2}+\frac{1}{\sigma_\omega^2}} \\
     \sigma_{M_{it}}^2 = \frac{1}{\frac{1}{\sigma_{M_{i,t-1}}^2}+\frac{1}{\sigma_\nu^2}} \\
     \sigma_{A_{it}}^2 = \frac{1}{\frac{1}{\sigma_{A_{i,t-1}}^2}+\frac{1}{\sigma_\varpi^2}} \\
     \sigma_{H_{it}}^2 = \frac{1}{\frac{1}{\sigma_{H_{i,t-1}}^2}+\frac{1}{\sigma_\upsilon^2}} \\
\end{aligned}
\end{equation}

\begin{equation}
\begin{aligned}
     \sigma_{Q_{it}}^2 = \frac{1}{ \frac{\phi^2}{\sigma_\eta^2+\sigma_\omega^2} + \frac{\varphi^2}{\sigma_\zeta^2+\sigma_\nu^2} + \frac{\psi^2}{\sigma_\varsigma^2+\sigma_\varpi^2} + \frac{\rho^2}{\sigma_\iota^2+\sigma_\upsilon^2} + \frac{1}{\sigma_{Q_{i,t-1}}^2}}
\end{aligned}
\end{equation}

At time $t$, the platform evaluates $i$'s loan application based on her updated belief of the applicant's quality $Q_{it}$. If the expected utility of approval is larger than zero, then the evaluator would approve $i$'s application. The utility is defined as:

\begin{equation}
\begin{aligned}
    u_{it} = z*(p_{it}a_{it}-(1-p_{it})b_{it})-c_{ig}+\epsilon_{it},
\end{aligned}
\end{equation}

\noindent where $g \in \{M, F\}$, $M$ stands for males and $F$ stands for females, $c_{ig}$ is the preference-based bias with $c_{i,g=M}=0$, $a_{it}$ is the money earned by the platform if non-default, $b_{it}$ is the money lost by the platform if default, $z$ is the price coefficient, and $r$ measures the risk aversion respect to the variation of credit quality. $p_{i}$ is the non-default probability of $i$ at time $t$, which is related to its quality $Q_{i,t-1}$ through a sigmoid function $h(x)=\frac{1}{1+\exp(-x)}$:

\begin{equation}
\begin{aligned}
    p_{it} = h(Q_{i,t-1}) = \frac{1}{1+\exp(-Q_{i,t-1})}.
\end{aligned}
\end{equation}
